# Supplementary material for: Graphons of Line Graphs
Source: arXiv:2409.01656 source file (2026-10-08)
Supplement: Supplementary file 1 [file 7_Appendix.tex]

% \pagebreak
% \appendix 
% \section{Proofs on sparse graphs with dense line graphs}\label{sec:appendix1}

% \corGnDense
% \begin{proof} 
% As $D \subset \bar{S}$, where $\bar{S}$ denotes the complement of $S$, this is true because of the contrapositive of Lemma \ref{lemmapropsparse}. It can be quickly verified that dense graph sequences do  not satisfy  equation \eqref{eq:sq2} in  Lemma \ref{lemmapropsparse} because for dense graphs  $m  \geq c n^2$ for some $c>0$.
% \end{proof}

% \lemmanotsqu*
% \begin{proof}
%     The first part is the contra-positive of Theorem \ref{thm:main}(2). We prove it from first principles for the sake of completeness. Let us restate the square-degree property and consider its negation. If a graph sequence $\{G_n\}_n$ satisfies the square-degree property, then there exists constants $c_1 \in (0,1)$ and $N_0 \in \mathbb{N}$ such that for all $n \geq N_0$ we have
%     $$ \sum \deg v_{i,n}^2 \geq c_1 \left( \sum \deg v_{i,n}\right)^2 \, . 
%     $$
%     The negation of square-degree property, $\neg Sq$ says that for all $c_1 > 0$ and $N_0 \in \mathbb{N}$ there exists $n \geq N_0$ such that 
%     $$ \sum \deg v_{i,n}^2 < c_1 \left( \sum \deg v_{i,n}\right)^2 \, . 
%     $$
%     For every $N_0 \in \mathbb{N}$ there exists $n \geq N_0$ such that this inequality is satisfied. Consider
%     $$ A_{c_1} = \left \{n \in \mathbb{N}: n \geq N_0, \sum \deg v_{i,n}^2 < c_1 \left( \sum \deg v_{i,n}\right)^2 \right\} \, . 
%     $$
%     If $|A_{c_1}|$ was finite, then we can pick $N_\nu = \max (A_{c_1}) + 1$ and for $n \geq N_{\nu}$ the inequality $\sum \deg v_{i,n}^2 < c_1 \left( \sum \deg v_{i,n}\right)^2$ would not be satisfied. Thus, the set $ A_{c_1} $ has infinitely many elements. Therefore for every $c_1 \in (0,1)$ and $N_0 \in \mathbb{N}$ there is an infinite sequence $A_{c_1}$ such that for any $n \in A_{c_1}$
%     $$ \sum \deg v_{i,n}^2 < c_1 \left( \sum \deg v_{i,n}\right)^2 \, . 
%     $$
%     Hence we can consider a sequence of sequences $\{ A_{c_{1_i}} \}_{c_{1_i}}$ where $c_{1_i} > c_{1_j}$ when $i < j$. From this sequence set we can choose a diagonal subsequence $\{n_1, n_2, \ldots \}$ such that $n_1 \in A_{c_{1_1}}$ and $n_2 \in A_{c_{1_2}}$ and so on, such that this sequence converges to zero. 
%     From equation~\eqref{eq:linedensity} recall that
%     $$ \density(H_m)  = \frac{\frac{1}{2}\sum_i (\deg\,  v_{i,n})^2 - m}{\frac{1}{2}m(m-1)} \, . 
%     $$
%     For the diagonal subsequence selected above
%     $$ \frac{ \sum \deg v_{i,n}^2}{\left( \sum \deg v_{i,n}\right)^2} = \frac{ \sum \deg v_{i,n}^2}{4m^2} \to 0 \, , 
%     $$
%     giving us
%     $$ \liminf_{m \to \infty}\density(H_{m}) = 0 \, . 
%     $$
%     If $\{H_m\}_m$ is convergent, then all subsequences converge to the same limit and we get
%     $$ \lim_{m \to \infty}\density(H_{m}) = 0 \, . 
%     $$
% \end{proof}

% \lemmahomedgedensity*
% \begin{proof}
% From Definition \ref{def:graphhomo}  
% \begin{equation}
%      t(F, H_m)   = \sum_{\phi: V(F) \to V(H_m)} \prod_{ij \in E(F)}  \beta_{\phi(i)\phi(j)}(H_m)  \cdot \frac{1}{m^{|V(F)|}} \, ,  \\
% \end{equation}    
% where $\phi$ is a mapping from $V(F)$ to $V(H_m)$ and $\beta_{ij}(H_m)$ denotes the weight of edge $ij$ in graph $H_m$, which is either 1 or 0. Thus, 
% \begin{align}
%     t(\edge, H_m)   & = \sum_{\phi: V(\edge) \to V(H_m)} \prod_{ij \in E(\edge)}  \beta_{\phi(i)\phi(j)}(H_m)  \cdot \frac{1}{m^{2}} \, ,  \\
%     & = \sum_{ \substack{ \phi: V(\edge) \to V(H_m) \\ ij \in E(\edge) }}  \beta_{\phi(i)\phi(j)}(H_m)  \cdot \frac{1}{m^{2}} \, ,
% \end{align}
% where we have dropped the product term as there is only one edge. We can replace the edge weight $\beta_{\phi(i)\phi(j)}(H_m)$ with the associated value in the empirical graphon $U_m(q_{\phi(i)}, q_{\phi(j)})$  giving us
% \begin{align}
%     t(\edge, H_m) & = \sum_{ \substack{ \phi: V(\edge) \to V(H_m) \\ ij \in E(\edge) }}   U_m(q_{\phi(i)}, q_{\phi(j)}) \cdot \frac{1}{m^2} \, ,  \\ 
%     & = \sum_{i,j} U_m(q_i, q_j) \cdot \frac{1}{m^2} \, , 
% \end{align}
% as $\phi$ can map the edge to any two vertices in $H_m$. Every edge in $G_n$ is mapped to a vertex in $H_m$ and 2 vertices in $H_m$ are connected if the corresponding edges in $G_n$ have a common vertex. That is, $L(\twoedges) = \edge $,  and for every edge in $H_m$ there is a corresponding set of two edges with a common vertex (\twoedges) in $G_n$. As a result the empirical graphon (Definition \ref{def:empiricalgraphon}), 
% $$ U_m(q_i, q_j) = 1 \quad \text{if and only if} \quad W_n(r_k, r_\ell)W_n(r_\ell, r_s) = 1
% $$
% for some $k, \ell, s \in  \{1, \ldots, n \}$ with $k \neq s$.  The reason $ k \neq s$ is because we need 2 distinct edges in $G_n$ with a common vertex to make an edge in $H_m$. As a result of this one-to-one and onto mapping we have
% \begin{equation}\label{eq:lemmahomdense1}
%     \sum_{i, j} U_m(q_i, q_j) = \sum_{ \substack{ k, \ell, s \\ k \neq s }} W_n(r_k, r_\ell)W_n(r_\ell, r_s)  \,  
% \end{equation}
% giving us the desired result. 
% \end{proof}


% \lemmadensegraphs*
% \begin{proof}
%     As $\{G_n\}_n$ is a dense graph sequence converging to $W$ 
% \begin{equation}\label{eq:lemmadense1}
%     \lim_{n \to \infty} t( \edge \, , G_n) = \lim_{n \to \infty} \frac{2m}{n^2}=  c > 0 \, .
% \end{equation}
% We will use this  limit later. Let $W_{n}$ be the empirical graphon of $G_n$ with $[0,1]$ divided into $n$ equal intervals $\{r_1, \ldots r_n \}$  and let $U_m$ be the empirical graphon of $H_m$ with $[0,1]$ equally divided into $m$ intervals $\{q_1, \ldots, q_m\}$. The homomorphism density $ \{t( \twoedges, G_n) \}_n$ is a converging sequence as $\{G_n\}_n$  converges to $W$. We have
% $$  t( \twoedges, G_n)  =  \sum_{\substack{ i, j, k   }}  W(r_i, r_k)W(r_k, r_j)\cdot \frac{1}{n^{3}} \, , 
% $$ % \\ i \neq j
% converging as $n$ goes to infinity.
% From Lemma \ref{lemma:homedgedensity} we know 
% % $$  t( F, H_m) =  \sum_{i, j \in V(F)} \prod_{\substack{ ij \in E(F) \\ i \neq j}} \sum_{k \in [n]} W(r_i, r_k)W(r_k, r_j)\cdot \frac{1}{m^{|V(F)|}} \, .
% % $$
% \begin{align}
%      t( \edge, H_m) & =   \sum_{\substack{ i, j  }}  U(q_i, q_j) \cdot \frac{1}{m^{2}} \, , \\ 
%       & =  \sum_{\substack{ i, j, k \\ i \neq j  }}  W(r_i, r_k)W(r_k, r_j)\cdot \frac{1}{m^{2}} \, ,  \\
%      & \leq \sum_{\substack{ i, j, k  }}  W(r_i, r_k)W(r_k, r_j)\cdot \frac{1}{m^{2}} \, , \\
%      & = \sum_{\substack{ i, j, k  }} \frac{1}{n^4} W(r_i, r_k)W(r_k, r_j)\cdot \frac{1}{ \left(\frac{m}{n^2} \right)^2 } \, .
% \end{align}
% As $n$ and $m$ go to infinity we get
% $$  \limsup_{m \to \infty}  t( \edge, H_m) = \lim_{\substack{ n \to \infty \\ m \to \infty} } \frac{1}{n} \cdot  t( \twoedges, G_n)  \cdot \frac{1}{ \left(\frac{m}{n^2} \right)^2 }  = 0 \, ,
% $$
% as $m/n^2$ goes to $c/2 > 0$ (equation \eqref{eq:lemmadense1}) and $t( \twoedges, G_n) $ converges. As $ t( \edge, H_m) $ lies between $0$ and $1$ we get
% $$  \lim_{m \to \infty}  t( \edge, H_m) = 0 \, . 
% $$
% As $t( \edge, H_m) = \frac{2m'}{n'^2}$ goes to 0, where $m'$ and $n'$ denote the number of edges and vertices in $H_m$, the cut-norm (Definition \ref{def:cut1}) satisfies
% $$ \lVert U_{H_m} - U \rVert_\square = \lVert U_{H_m} \rVert_\square  = \frac{2m'}{n'(n'-1)}  \rightarrow 0 \, , 
% $$
% where $U(x,y) = 0$.   As the cut-metric (Definition \ref{def:cut2})
%     $$ \delta_\square \left(U_{H_m}, U \right) = \inf_{\varphi} \lVert U_{H_m} - U^{\varphi} \rVert \, , 
%     $$
%    $\{H_m\}_m$ converges to $U$ in the cut-metric as the infimum is considered and as $U^{\varphi} = U$ for $U = 0$. 
% \end{proof}


% \lemmaconverginginSq*
% \begin{proof}
%  From Theorem \ref{thm:main} we know $\{G_n\}_n\in S_q \equiv \{H_m\}_m \in D$. Additionally, if $\{H_m\}_m$ converges to $U$ then $\{ t(\edge, H_m)\}_m$  converges to $t(\edge, U)$. As $t(\edge, H_m) = \frac{2m'}{n'^2}$ where $m'$ and $n'$ denote the number of edges and nodes in $H_m$ where $n' = m$, the sequence $\frac{2m'}{n'^2}$ converges to some constant $c$. But as $\{H_m\}_m \in D$ 
%  $$ t(\edge, U) =  \lim_{n' \to \infty} \frac{2m'}{n'^2} = c > 0 \, ,
%  $$
% that is, the edge density of $\{H_m\}_m$ converges to a positive constant. The homomorphism density $t(\edge, U)$ (Definition \ref{def:graphhomo}) is given by
%  $$ t(\edge, U) = \int_{[0,1]^2} U(x, y) \, dx dy   \, , 
%  $$
% which is equal to the cut-norm of $U$
% $$  \lVert U \rVert_\square = \sup_{S ,T} \left \vert \int_{S \times T} U(x,y) dxdy \right\vert \, , 
% $$
% because $U(x,y) \in [0,1]$ and the supremum is achieved when $S = T = [0,1]$, giving us 
% $$ \lVert U \rVert_\square  =  t(\edge, U)  > 0 \, . 
% $$
%  % Let $\{G_n\}_n\in S$ be a sparse graph sequence. Let $\{H_m\}_m$ be the corresponding sequence of line graphs with $H_m = L(G_n)$. Then $\{G_n\}_n\in S_q \equiv \{H_m\}_m \in D$, i.e., $\{G_n\}_n$ satisfies $Sq$ if and only if $\{H_m\}_m$ is dense. 
% \end{proof}


% \lemmaconvergingSnotSq*
% \begin{proof}
%     As $\{G_n\}_n \in S$, it is sparse and it converges to $W = 0$.  From Lemma \ref{lemma:notsqu}\,  if  $\{G_n \}_n \notin S_q$ 
%       $$ \liminf_{m \to \infty}\density(H_{m}) = 0 \, . 
%     $$
%     As $\{H_m\}_m$ converges to $U$, the edge densities converge and we get $\lim_{m \to \infty} \density(H_m) = 0$. 
%     The empirical graphon $U_{H_m}$ converges to $U$ and we have the cut norm (Definition \ref{def:cut1}) of the empirical graphon
%     $$ \lVert U_{H_m} \rVert  = \frac{2m'}{n'(n'-1)} \to 0
%     $$
%     giving us 
%     $$ \lim_{m \to \infty}   \lVert U_{H_m} - U \rVert = 0 \, , 
%     $$
%     where $U = 0$. As the cut-metric (Definition \ref{def:cut2})
%     $$ \delta_\square \left(U_{H_m}, U \right) = \inf_{\varphi} \lVert U_{H_m} - U^{\varphi} \rVert \, , 
%     $$
%     we get the result. 
% \end{proof}

% \lemmaWandU*
% \begin{proof}
%     For  converging sequences $\{ G_n\}_n$ and  $\{ H_m\}_m$ we have $W = 0$ or $U = 0$ (Lemmas \ref{lemma:densegraphs}, \ref{lemma:converginginSq} and \ref{lemma:convergingSnotSq}).  The graphon $W \neq 0$ only when $\{G_n\}_n \in D$. When $\{G_n\}_n \in D$ we have $\{H_m\}_m \in S$ giving $U = 0$. The graphon $U \neq 0 $ only when $\{G_n\}_n \in S_q$ implying $W = 0$ as $S_q \subset S$. %Figure \ref{fig:mappingWtoU} explains this Lemma. 
% \end{proof}


%\section{Proofs on results for deterministic graphs}
% \lemmastargraphsone*
% \begin{proof}
%    We present an alternate proof from first principles.
%    For the sake of completeness, we do the computation from first principles. For a star graph 
%        $$ \deg v_i =  \begin{cases} 
%       n-1 \quad \text{ for star vertex } \, , \\
%       1 \quad \text{otherwise} 
%    \end{cases}
%        $$
%  giving us       
%     \begin{align*}
%         \sum \deg v_{i,n}^2 & = (n-1)^2 + 1 + \cdots + 1 \, ,  \\
%         & = (n-1)^2 + (n-1) \, , \\
%         \sum \deg v_{i,n} & = m = n-1  \, ,  \\
%         \frac{\sum \deg v_{i,n}^2}{\left( \sum \deg v_{i,n} \right)^2} & = 1 + \frac{1}{n-1} > 1 \, ,   
%     \end{align*}
%  showing that  $\{K_{1,n}\}_n \in S_q$ (Definition \ref{def:square}). From equation \eqref{eq:linedensity}, the density of $H_m$ is given by
%    \begin{align*}
%         \density(H_m) & = \frac{\frac{1}{2}\sum_i (\deg\,  v_{i,n})^2 - m}{\frac{1}{2}m(m-1)} \, , \\
%         & = \frac{\frac{1}{2}( (n-1)^2 + 1 +1 + \ldots + 1 ) - (n -1)}{ \frac{1}{2} (n-1)(n-2)} \, ,  \\
%         & = \frac{ \frac{1}{2}((n-1)^2 + (n-1) ) - (n-1) }{\frac{1}{2}(n-1)(n-2)} \, ,  \\
%         & = \frac{\frac{1}{2}(n-1)(n) - (n-1)}{\frac{1}{2}(n-1)(n-2)}  \, , \\
%         & = \frac{\frac{1}{2}(n-1)(n-2)}{\frac{1}{2}(n-1)(n-2)} \, , \\
%         & = 1\, . 
%    \end{align*}   
%    Thus, $\lim_{m \to \infty}\density(H_m)  = 1$. 
% \end{proof}

% \lemmastargraphontwo*
% \begin{proof}
%     The line graph of $k$ disjoint stars is $k$ disjoint complete subgraphs.  This follows from Lemma \ref{lemma:linegraphs} (\ref{lemma:linegraphs:connectedgraph} and \ref{lemma:linegraphs:star}) as vertices of 2 different stars are not connected. Noting $H_{m_i}$ has $m_i$ vertices, we obtain the empirical graphon (Definition~\ref{def:empiricalgraphon}) of $H_{m_i}$ by splitting the interval $[0, 1]$ into $m_i$ equal intervals $\{I_1, I_2, \ldots, I_{m_i} \}$. 
    
%     At the $i$th step, the $j$th star $K_{1, s_j}$ has $1 + i r_j$ nodes and $ir_j$ edges. Then the corresponding complete subgraph $K_{s_j} $ of the line graph $H_{m_i}$ has $i r_j$ nodes as each node in the line graph corresponds to an edge in $G_{n_i}$. We label nodes belonging to a complete subgraph consecutively. That gives us vertices $1, \ldots , ir_1$ corresponding to the first complete subgraph $K_{s_1}$, and nodes $(ir_1+ 1), \ldots,  (ir_1 + ir_2)$ corresponding the second complete subgraph $K_{s_2}$ and so on. The ratio between the number of nodes in each subgraph is $r_1:r_2:\ldots:r_k $. 

%     Let us group the vertices in $H_m$,  $\{1, 2, \ldots, {m_i} \}$ into $k$ groups $\{J_1, J_2, \ldots, J_k \}$ according to the complete subgraph they belong to. Then for $x \in I_j, y \in I_h$ we have the empirical graphon (Definition \ref{def:empiricalgraphon}) of $H_m$
%     $$ U_{H_{m_i}}(x,y) = \begin{cases} 
%       1 \quad \text{if} \quad  j, h \in J_\ell \text{ for some } \ell  \text{ but } j \neq h  \\  
%       0 \quad  \text{if} \quad j = h \text{ as there are no loops} \\
%       0 \quad \text{if} \quad  j \in J_p \text{ and } h \in J_q \text{ where } p \neq q
%     \end{cases} \, .
%     $$

% The bottom row in Figure~\ref{fig:1to4stars} shows empirical graphons for $k \in \{2, 3, 4\}$.
% Note that $U$ is a block diagonal graphon similar to $U_{H_{m_i}}$ differing to $U_{H_{m_i}}$ only on the diagonal. One can visualize $U$ by colouring the white squares on the diagonal in empirical graphons in  Figure~\ref{fig:1to4stars} for $k \in \{2, 3, 4\}$. 

% Then, the cut-norm (Definition~\ref{def:cut1}), 
%  \begin{align}
%      \lVert U_{H_m}  - U\rVert_\square &= \sup_{S, T} \left\vert\int_{S\times T} U_{H_m}(x,y)  - U(x,y) \, dx dy \right\vert  \, \, , \\
%      & =  \frac{1}{m_i^2} \times m_i = \frac{1}{m_i} \, ,  
%  \end{align}
%  %  That is, 
% %  $$ \lVert U_{H_{m_i}} - U \rVert_\square = \frac{1}{m_i^2} \times m_i = \frac{1}{m_i} \, ,  
% %  $$
% % where we have used $S = T = [0,1]$ in computing the cut-norm 
% % $$ \lVert U_{H_m}  - U\rVert_\square = \sup_{S, T} \left\vert\int_{S\times T} U_{H_m}(x,y)  - U(x,y) \, dx dy \right\vert  \, \, ,
% % $$
% where we have used $S = T = [0,1]$ in computing the cut-norm as any other $S$ or $T$ would give smaller area. Then the cut metric (Definition~\ref{def:cut2})
% $$ \delta_{\square}( U_{H_m}, U) = \inf_\varphi \left\lVert  U_{H_m} - U^\varphi \right\rVert_\square  \leq  \lVert U_{H_m}  - U\rVert_\square  = \frac{1}{m_i} \, .
% $$
% As $ \lVert U_{H_m}  - U\rVert_\square $ goes to zero as $m$ goes to infinity $\delta_{\square}( U_{H_m}, U) $ converges to zero.  From Theorem \ref{thm:BCconvergent2} \citep{borgs2011limits} $\{H_{m_i}\}_{m_i}$ converges to $U$.
% \end{proof}


% \thmproplinegraphs*
% \begin{proof}
% Recall that 
% $$    \density(H_m) = \frac{\frac{1}{2}\sum (\deg\,  v^2) - m}{\frac{1}{2}m(m-1)} \, . 
% $$
%     \begin{enumerate}
%         \item Suppose $G_n$ is the complete graph $K_n$. As $\density(K_n) = 1$, the sequence $\{K_n\}_n$ is dense, i.e, $ \{K_n\}_n \in D$. For $K_n$,  $\deg v_i = n-1$ and $m = n(n-1)/2$ giving us
%         \begin{align*}
%          \density(H_m) & = \frac{\frac{1}{2} n(n-1)^2 - \frac{1}{2}n(n-1) }{ \frac{1}{2} \frac{1}{2}n(n-1)(\frac{1}{2}n(n-1) - 1) } \, ,  \\
%          & = \frac{\frac{1}{2} n(n-1)(n-1 -1)}{\frac{1}{2} \frac{1}{2}n(n-1)\frac{1}{2}(n(n-1) - 2)} \\
%          & =  \frac{n-2}{ \frac{1}{4} (n+1)(n-2) } \, , \\
%          & = \frac{4}{n + 1} \, , \\
%       \text{making} \quad   \lim_{m \to \infty}\density(H_m) & = 0  \Rightarrow \{H_m\}_m \in S.  
%         \end{align*}
%    % We can also show this using Lemma \ref{lemma:linegraphs}-\ref{lemma:linegraphs:r-regulargraph}. When $G_n$ is complete,  $H_m$ is a $2(n-2)$-regular graph with $m =n(n-1)/2 $ vertices making the density of the line-graphs tend to zero. %Thus, $\{G_n\}_n \in D$ and $\{H_m\}_m \in S$.  %, the graphon $W(x,y) = 0$ as well. 
        
%        \item  Suppose $G_n$ is an $r$-regular graph. As $n$ grows each $G_n$ is connected to $r$ nodes.   Then $\deg v_i = r$ and $m = rn/2$. The ratio $m/n^2 = r/2n$ assigning $\{G_n\}_n \in S$. %As each node has the same degree in $G_n$ it does not satisfy the square-degree property, i.e. $\{G_n\}_n \in S \backslash S_q$.
%        The density of $H_m$ is given by
%        \begin{align}
%             \density(H_m) & = \frac{ \frac{1}{2}nr^2 - \frac{1}{2}nr }{ \frac{1}{2}   \frac{1}{2} rn   ( \frac{1}{2} rn - 1 )  } \, ,  \\
%             & = \frac{ \frac{1}{2}rn(r-1)}{ \frac{1}{2} \frac{1}{2} rn \frac{1}{2}(rn -2 )} \, ,  \\
%             & = \frac{4(r-1)}{rn - 2} \, , \\
%             & = \frac{2(r-1)}{m - 1} \, . 
%             \label{eq:linedensityrregular} 
%        \end{align}
%      Thus, $\lim_{m \to \infty}\density(H_m) = 0$, making both $\{G_n\}_n, \{H_m\}_m \in S$. 
%     Using Theorem \ref{thm:main} we can conclude $\{G_n\}_n \notin S_q$ because  $\{G_n\}_n \in S_q  \iff \{H_m\}_m \in D$. Hence $\{G_n\}_n \in S\backslash S_q$.  
%      As $G$ is an $r$-regular graph, $H$ is a $2(r-1)$-regular graph with $\frac{nr}{2}$ vertices (Lemma \ref{lemma:linegraphs}-\ref{lemma:linegraphs:r-regulargraph}).  Thus, using the same reasoning we have $\{H_m\}_m \in S\backslash S_q$.   
%      This is an example where both graph sequences $\{G_n\}_n$ and $\{H_m\}_m$ are sparse and both $\{G_n\}_n, \{H_m\}_m \in S\backslash S_q$.  % and $W(x,y) = 0$. 
%    %     \item Suppose $G_n$ is a star. Then $H_m$ is a complete graph (Lemma \ref{lemma:linegraphs}). This gives us the desired result. Or we can do the computation from first principles. For a star graph 
%    %     $$ \deg v_i =  \begin{cases} 
%    %    n-1 \quad \text{ for star vertex } \, , \\
%    %    1 \quad \text{otherwise} 
%    % \end{cases}
%    %     $$
%    %    and $m = n-1$ giving us
%    % \begin{align*}
%    %      \density(H_m) & = \frac{\frac{1}{2}( (n-1)^2 + 1 +1 + \ldots + 1 ) - (n -1)}{ \frac{1}{2} (n-1)(n-2)} \, ,  \\
%    %      & = \frac{ \frac{1}{2}((n-1)^2 + (n-1) ) - (n-1) }{\frac{1}{2}(n-1)(n-2)} \, ,  \\
%    %      & = \frac{\frac{1}{2}(n-1)(n) - (n-1)}{\frac{1}{2}(n-1)(n-2)}  \, , \\
%    %      & = \frac{\frac{1}{2}(n-1)(n-2)}{\frac{1}{2}(n-1)(n-2)} \, , \\
%    %      & = 1\, . 
%    % \end{align*}   
%    % Thus, $\lim_{m \to \infty}\density(H_m)  = 1$. As the line graph of a star is a complete graph, the adjacency matrix consists of all ones apart from the diagonal  making $U(x,y) = 1$ for all $x$ and $y$.  For star graphs $\{G_n\}_n \in S_q$ and $\{H_m\}_m \in D$.
%    \item Suppose $G_n$ is a path. Then $m = n-1$ and the starting and ending vertices have degree 1 and the rest have degree 2. Thus, 
%     \begin{align*}
%         \density(H_m) & = \frac{\frac{1}{2} (1^2 + (n - 2)2^2 + 1 ^2) - m }{\frac{1}{2}m(m-1)} \, , \\
%         & = \frac{\frac{1}{2}(2 + 4(m-1)) - m}{\frac{1}{2}m(m-1)} \, ,  \\
%         & =  \frac{1 + 2(m-1) - m}{\frac{1}{2}m(m-1)} \, ,  \\
%         & = \frac{m-1}{\frac{1}{2}m(m-1)}  \, , \\
%         & = \frac{2}{m} = \frac{2}{n-1} \, . 
%     \end{align*}
%     Thus, $\lim_{m \to \infty}\density(H_m)  = 0$. 
%     The edge density can also be derived by recognizing a path of $n$ vertices gives rise to a line graph that is a path of $n-1$ vertices (Lemma~\ref{lemma:linegraphs}-\ref{lemma:linegraphs:paths}). 
%     %In the above computation we used equation \eqref{eq:linedensity} to obtain the result. 
%     Using the same reasoning as previously for $r$-regular graphs, we can conclude that both $\{G_n\}_n, \{H_m\}_m \in S\backslash S_q$.    %making $W(x,y) = 0$ for all $x$ and $y$. T

%     \item Suppose $G_n$ is a cycle, i.e. $G_n = C_n$. Then $n = m$ and all vertices have degree 2. This is a 2-regular graph. Using equation \eqref{eq:linedensityrregular} we get
%     \begin{align}
%           \density(H_m) & = \frac{4(r-1)}{rn - 2} \, , \\
%            & = \frac{4}{2n - 2}  = \frac{2}{n-1} = \frac{2}{m-1} \, , 
%     \end{align}
%     which limits to zero. From Lemma \ref{lemma:linegraphs}-\ref{lemma:linegraphs:cyle} we know that $L(C_n) = C_n$. 
%     Here too both $\{G_n\}_n, \{H_m\}_m \in S\backslash S_q$ as previously.    % with $W = 0$. 
% \end{enumerate}
% \end{proof}

% \section{Proofs on results for probabilistic graphs}
% \begin{lemma}\label{lemma:erdospartresult1}
% Consider the graph $G_n $ sampled from a $G(n,p)$ model and suppose $G_n$ has $n$ nodes and $m$ edges. Let $X_{ij}$ denote the random variable corresponding to the edge between vertices $i$ and $j$, i.e., $X_{ij} = 1$ if the edge exists and $0$ otherwise. Let $Y_j = \sum_i X_{ij}$,  $\mu = \mathbb{E}[Y_j]$ and $\bar{m} = \mathbb{E}[m]$. Let $Y_{\ssq} = \sum_j Y_j^2$, and $m_{\sq} = m^2$. Then for a given $\alpha \in (0,1)$ and $c > 0$ we have
% \[
% P\left[ Y_{\ssq}\geq c m_{\sq} \vert m_{\sq}  \leq (1 - \alpha)^2\bar{m}^2  \right] P\left[ m_{\sq} \leq (1 - \alpha)^2\bar{m}^2  \right] \leq \exp\left( - \frac{\alpha^2 pn(n-1)}{4} \right) \, . 
% \]
% \end{lemma}
% \begin{proof}
% For a given $\alpha \in (0,1)$ we get the following Chernoff-Hoeffding bounds \citep{Frieze2015book} for $m$:
% \begin{align}
%       P \left[m \leq (1 - \alpha)\bar{m} \right] & \leq \exp\left( - \frac{\alpha^2 \bar{m}}{2} \right) \, ,  \label{eq:erdosrenyi6} \\
%   \text{giving us } \quad        P\left[m^2 \leq (1 - \alpha)^2\bar{m}^2 \right] & \leq \exp\left( - \frac{\alpha^2 \bar{m}}{2} \right) \, ,  \label{eq:erdosrenyi7}   
% \end{align} 
% as $m$ is positive.  As the probability $P\left[ Y_{\ssq}\geq c m_{\sq} \vert m_{\sq}  \leq (1 - \alpha)^2\bar{m}^2  \right] \leq 1$, $m_{\sq} = m^2$ and  $\bar{m} = pn(n-1)/2$ we get the desired result. 
% \end{proof}


% \begin{lemma}\label{lemma:erdospartresult2}
% Consider the graph $G_n $ sampled from a $G(n,p)$ model and suppose $G_n$ has $n$ nodes and $m$ edges. Let $X_{ij}$ denote the random variable corresponding to the edge between vertices $i$ and $j$, i.e., $X_{ij} = 1$ if the edge exists and $0$ otherwise. Let $Y_j = \sum_i X_{ij}$,  $\mu = \mathbb{E}[Y_j]$ and $\bar{m} = \mathbb{E}[m]$. Let $Y_{\ssq} = \sum_j Y_j^2$, and $m_{\sq} = m^2$. Then for a given $\alpha \in (0,1)$ and $c > 0$ we have
% \[
% P\left[ Y_{\ssq}\geq c m_{\sq} \vert m_{\sq}  \geq (1 + \alpha)^2\bar{m}^2  \right] P\left[ m_{\sq} \geq (1 + \alpha)^2\bar{m}^2  \right] \leq \exp\left( - \frac{\alpha^2 pn(n-1)}{6} \right) \, . 
% \]
% \end{lemma}
% \begin{proof}
%     The proof is similar to Lemma \ref{lemma:erdospartresult1} with the only difference being the Chernoff-Hoeffding bound, which changes to:
% $$  P\left[m \geq (1 + \alpha)\bar{m} \right]  \leq \exp\left( - \frac{\alpha^2 \bar{m}}{3} \right) \, . 
% $$
% \end{proof}

% \begin{lemma}\label{lemma:erdospartresult3}
% Consider the graph $G_n $ sampled from a $G(n,p)$ model and suppose $G_n$ has $n$ nodes and $m$ edges. Let $X_{ij}$ denote the random variable corresponding to the edge between vertices $i$ and $j$, i.e., $X_{ij} = 1$ if the edge exists and $0$ otherwise. Let $Y_j = \sum_i X_{ij}$,  $\mu = \mathbb{E}[Y_j]$ and $\bar{m} = \mathbb{E}[m]$. Let $Y_{\ssq} = \sum_j Y_j^2$, and $m_{\sq} = m^2$. Then for a fixed $c >0$ and fixed $\alpha \in (0,1)$ for $n > \frac{4}{c(1-\alpha)^2}$ and $\beta = \frac{\sqrt{cn}(1 - \alpha)}{2} - 1$ we have
% \begin{align}
%     P\left[ Y_{\ssq}\geq c m_{\sq} \vert  (1 - \alpha)^2\bar{m}^2 \leq  m_{\sq} \leq  (1 + \alpha)^2\bar{m}^2 \right] & P\left[ (1 - \alpha)^2\bar{m}^2 \leq  m_{\sq} \leq  (1 + \alpha)^2\bar{m}^2  \right]  \\
%     & \leq \exp\left(\ln n - \frac{\beta^2 p (n-1)}{3} \right) \, . 
% \end{align}
% \end{lemma}
% \begin{proof}
%     We focus on the term $ P\left[ Y_{\ssq}\geq c m_{\sq} \vert  (1 - \alpha)^2\bar{m}^2 \leq  m_{\sq} \leq  (1 + \alpha)^2\bar{m}^2 \right]$. We know that $\mu = p(n-1)$ and $\bar{m} = pn(n-1)/2$.  As $ m_{\sq} \in \left[ (1 - \alpha)^2\bar{m}^2, \,   (1 + \alpha)^2\bar{m}^2 \right]$ we get
% \begin{align}
%     P\left[ Y_{\ssq}\geq c m_{\sq} \vert  (1 - \alpha)^2\bar{m}^2 \leq  m_{\sq} \leq  (1 + \alpha)^2\bar{m}^2 \right] & \leq P\left[ Y_{\ssq}\geq c(1 - \alpha)^2\bar{m}^2 \right] \, , \label{eq:erdosrenyi10} \\
%    & = P\left[ Y_{\ssq} \geq c\left( \frac{n\mu}{2} \right)^2 (1 - \alpha)^2  \right]  \, , \label{eq:erdosrenyi11} \\
%    & =  P\left[  Y_{\ssq} \geq n \mu^2 (1 + \beta)^2\right] \, , \label{eq:erdosrenyi12} 
% \end{align} 
% where we have substituted  $\bar{m} = \frac{n \mu}{2}$ in equation \eqref{eq:erdosrenyi11}  and rearranged the terms for $\beta$. For $n > \frac{4}{c(1 - \alpha)^2}$, we get $\frac{\sqrt{cn}(1 - \alpha)}{2} > 1$ making $\beta > 0$. 

%  For a given $\beta > 0$, we get the following Chernoff-Hoeffding bound for $Y_j$:
%     \begin{align}
%         P\left[Y_j \geq (1 + \beta) \mu \right] \leq \exp \left( -\frac{\beta^2 \mu}{3}\right) \, .  \label{eq:erdosrenyi1}\\
%      %\cheng{Some more words about which properties enable this and the next step}} \\ 
%       \text{As } Y_j \geq 0 \text{ we have }  \quad   P\left[Y_j^2 \geq (1 + \beta)^2 \mu^2 \right] \leq \exp \left( -\frac{\beta^2 \mu}{3}\right) \, ,  \label{eq:erdosrenyi2} \\
%    \text{and from Boole's inequality} \quad        P\left[Y_{\ssq} \geq n(1 + \beta)^2 \mu^2 \right] \leq n \exp \left( -\frac{\beta^2 \mu}{3}\right) \, .  \label{eq:erdosrenyi3} \\        
%     \end{align}
% Substituting equation \eqref{eq:erdosrenyi3} in equation \eqref{eq:erdosrenyi12}  we get
% \begin{align}
%     P\left[ Y_{\ssq}\geq c m_{\sq} \vert  (1 - \alpha)^2\bar{m}^2 \leq  m_{\sq} \leq  (1 + \alpha)^2\bar{m}^2 \right] & \leq n \exp \left( -\frac{\beta^2 \mu}{3}\right) \, , \\
%     & \leq  \exp \left( \ln n -\frac{\beta^2 \mu}{3}\right)
% \end{align}
% for $n > \frac{4}{c(1-\alpha)^2}$ and $\beta = \frac{\sqrt{cn}(1 - \alpha)}{2} - 1$. 
% \end{proof}


% \thmerdosrenyi*
% \begin{proof}
%     Let $X_{ij}$ denote the Bernoulli random variable corresponding to the edge between nodes $i$ and $j$ in $G_n$ and let $X_{ij} = 1$ if the edge is present and $0$ otherwise. Let $Y_j = \sum_i X_{ij}$. Then the degree of each node $j$ in $G_n$ is given by $\deg v_j = Y_j$. Let $\mu = \mathbb{E}[Y_j]$ and $\bar{m} = \mathbb{E}[m]$. We know that $\mu = p(n-1)$ and $\bar{m}  = pn(n-1)/2$. Let $Y_{\ssq} = \sum_j Y_j^2$, and $m_{\sq} = m^2$ where ssq denotes the  sum of squares and sq denotes square.
    
% We fix $c$ and $\alpha$ such that $c, \alpha \in (0,1)$ and  compute $P\left[ Y_{\ssq} \geq c m_{\sq} \right]$ using the law of total probability 
% \begin{align}
%     P\left[ Y_{\ssq} \geq  c m_{\sq} \right]  & = P\left[ Y_{\ssq}\geq c m_{\sq} \vert m_{\sq}  \leq (1 - \alpha)^2\bar{m}^2  \right] P\left[ m_{\sq} \leq (1 - \alpha)^2\bar{m}^2 \right]  + \\
%     & \hspace{-1.5cm} P\left[ Y_{\ssq}\geq c m_{\sq} \vert  (1 - \alpha)^2\bar{m}^2 \leq  m_{\sq} \leq  (1 + \alpha)^2\bar{m}^2 \right] P\left[ (1 - \alpha)^2\bar{m}^2 \leq  m_{\sq} \leq  (1 + \alpha)^2\bar{m}^2  \right]  + \\
%     & \hspace{-1.5cm} P\left[ Y_{\ssq}\geq c m_{\sq} \vert m_{\sq} \geq (1 + \alpha)^2\bar{m}^2  \right] P\left[ m_{\sq} \geq (1 +  \alpha)^2\bar{m}^2 \right]  \, , \ \label{eq:erdosrenyi8} \\ 
%     & \leq \exp\left( - \frac{\alpha^2pn(n-1) }{4} \right) + \exp \left( \ln n -\frac{\beta^2 p(n-1)}{3}\right) + \exp\left( - \frac{\alpha^2pn(n-1)}{6} \right) \, ,  \label{eq:erdosrenyi9}
%  \end{align}   
% from Lemmas \ref{lemma:erdospartresult1}, \ref{lemma:erdospartresult2} and \ref{lemma:erdospartresult3} for $n > \frac{4}{c(1-\alpha)^2}$ and $\beta = \frac{\sqrt{cn}(1 - \alpha)}{2} - 1$.     

% For a fixed $c \in (0,1) $ we get
% $$ \lim_{n,m \to \infty}  P\left[ Y_{\ssq} \geq  c m_{\sq} \right]  = 0
% $$ 
% As 
% $$ P\left[ \frac{1}{2} Y_{\ssq} \geq  \frac{1}{2} c m_{\sq} \right] = P\left[\frac{1}{2}\sum_j Y_j^2  - m \geq  \frac{1}{2} c m^2 -m  \right]
% $$
% For $c \in (0,1)$ we have $ \frac{1}{2}cm^2 - \frac{1}{2}cm > \frac{1}{2}cm^2 - m$ giving us
% $$
% P\left[\frac{1}{2}\sum_j Y_j^2  - m \geq  \frac{1}{2} c m^2 - \frac{1}{2} c m  \right] \leq P\left[\frac{1}{2}\sum_j Y_j^2  - m \geq  \frac{1}{2} c m^2 -m  \right] =  P\left[ Y_{\ssq} \geq  c m_{\sq} \right] \, . 
% $$
% This gives us
% \begin{align}
% P\left[ \frac{\frac{1}{2}\sum_j Y_j^2  - m }{\frac{m(m-1)}{2}}   \geq c \right] & \leq P\left[ Y_{\ssq} \geq  c m_{\sq} \right]     \, , \\
%  P\left[ \density(H_m) \geq c \right]  & \leq  \exp\left( - \frac{\alpha^2pn(n-1) }{4} \right) + \exp \left( \ln n -\frac{\beta^2 p(n-1)}{3}\right) + \exp\left( - \frac{\alpha^2pn(n-1)}{6} \right) \, ,
% \end{align}
% where we have used the line graph edge density in equation \eqref{eq:linedensity}. 
% As $n$ and $m$ go to infinity
% % \begin{align}
% %    \lim_{n, m \to \infty} P\left[ \frac{\frac{1}{2}\sum_j Y_j^2  - m }{\frac{m(m-1)}{2}}  \geq c \right] & = 0 \, .   \\
% % \end{align}
% % Using the line graph edge density in equation \eqref{eq:linedensity}
% \begin{align}
%    \lim_{m \to \infty} P\left[ \density(H_m) \geq c \right] & = 0 \, , 
% \end{align}
% giving us the first result. 
% %obtaining equation \eqref{eq:result1erdosrenyithm}.
% Taking the complement we have
% $$  
%       \lim_{m \to \infty} P\left[ \density(H_m) < c \right] = 1\, ,
% $$
% for a fixed $c \in (0, 1)$. As this is true for any $c \in (0, 1)$ we have
% $$  \lim_{m \to \infty} P\left[ \density(H_m) = 0 \right] = 1\, . 
% $$
% \end{proof}  
